# Supplementary material for: Re-Align: Structured Reasoning-guided Alignment for In-Context Image Generation and Editing
Source: arXiv:2601.05124 source file (2026-01-08)
Supplement: Supplementary file 1 [file X_suppl.tex]

\clearpage
\setcounter{page}{1}
\maketitlesupplementary
\appendix

\section{Model Architecture}
Our foreground-aware NeRF is constructed on Instant-NGP~\cite{muller2022instant} with an additional head to predict the editing probability to conduct decomposed rendering.
For simplicity in implementation, this editing probability head is designed similarly to the RGB prediction head.
It is composed of a hidden layer with 64 hidden dimensions followed by the sigmoid activation to keep the values between 0 and 1.
When rendering the foreground or background regions separately, we avoid truncating the editing probability gradient with the threshold operation.
Instead, we encourage the editing probability to approach 1 or 0 through a parameterized sigmoid activation and utilize the processed probabilities for decomposed rendering via a simple linear combination.
We find that this soft mask operation better facilitates complete shape optimization during the editing process compared to a threshold operation, as demonstrated by the ablation study presented in Section~\ref{sec:m_abla}.

\section{Implementation Details}

\noindent \textbf{Dataset preparation.}
In this paper, we conduct different editing operations using datasets such as BlendedMVS~\cite{yao2020blendedmvs} and LLFF~\cite{mildenhall2019local}. 
For 360-degree scenes from these datasets, we employ COLMAP~\cite{schoenberger2016sfm} to extract camera poses. 
This method can also be applied to real-world scenes captured by users.

\noindent \textbf{Rendering.}
Due to the memory limitation of the GPU and the high overhead of SDS loss, we need to render downsampled images.
For the BlendedMVS dataset, we render images with 3x downsampling for NeRF training and 5x downsampling for NeRF editing.
For the high-resolution LLFF and IBRNet~\cite{wang2021ibrnet} datasets, the two downsampling factors are 15 and 28.
For the bear statue dataset~\cite{in2n}, the two downsampling factors are 4 and 7.
Since we render the foreground for a separate local editing operation, we combine the rendered foreground image with a random solid color background to avoid confusion between the foreground and the single background of the same color.

% \noindent \textbf{Hybrid prompt generation.} 
% In image-driven editing, apart from manually inputting hybrid prompts that align with the image content, we can also employ models like GPT-4 to describe the contents of the original scene. 
% To ensure that the generated descriptions adhere to our required format, we specify the output format as ``[describe the subject] in [describe the environment]'', and replace the subject part of the obtained description with ``V* [cls]''. 
% Through this method, in image-driven editing, users only need to provide a reference image, eliminating the need for additional textual input to describe the original scene.

\section{More Ablation Studies}
\label{sec:m_abla}

\noindent \textbf{Visualization of intermediate results.}
We present the rendered editing probabilities and foreground/background images in Figure~\ref{fig:inter} after editing. 
It can be observed that the rendered editing probabilities can adapt well to the shape of the modified foreground regions, enabling the precise rendering of both foreground- and background-only images.
For instance, after the training process of the edited NeRF, the editing probability aligns well with the cartoon dinosaur, which is larger than the original dinosaur statue.
In the background image in the second row, we observe dark shadows in the foreground region, which indicates that NeRF does not picture the covered background regions in non-360 scenes. 
However, in the full rendering image, this shadow will be filled with foreground contents when the new objects being added are similar in shape to the original objects.

\begin{figure}[!htbp]
    \centering
    \includegraphics[width=\linewidth]{sec/figure/intermediate.pdf}
    \caption{Visualization of intermediate results.}
    \label{fig:inter}
\end{figure}

\noindent \textbf{Ablation studies of other training strategies.}
We conduct more ablation studies on training strategies in Figure~\ref{fig:abla}.
Upon removal of the background preservation loss, significant changes can be observed in the background regions after editing compared with the original scene, indicating the necessity of the background preservation loss.
We also ablate different post-processing methods for editing probabilities. 
When binarizing these probabilities using a threshold (i.e., w/o Soft Mask), the obtained editing probabilities are incomplete, leading to incomplete foreground in the edited results, such as the missing left front leg of the dog in the 3-rd row of Figure~\ref{fig:abla}. 
By scaling the values between 0 and 1 using a sigmoid function to obtain a soft mask, \textit{i.e.}, the strategy adopted in our paper, we can achieve complete editing probabilities and consequently, complete editing results.

\noindent \textbf{Effect of different class word.}
We use the class word in the local editing stage to promote reasonable geometry in the case of a single reference image. 
In order to explore the effect of the class word, we modify the class prior to be inconsistent with the reference image. 
As shown in Figure~\ref{fig:cls}, we compare different class words such as ``dog'', ``corgi'', and ``cat''. The final results reflect the texture of the reference image and the geometric characteristics associated with the class word we use.

\begin{figure}[!htbp]
    \centering
    \includegraphics[width=\linewidth]{sec/figure/abla.pdf}
    \caption{Ablation studies of other training strategies. w/o Soft Mask denotes utilizing a threshold to binarize the editing probabilities.}
    \label{fig:abla}
\end{figure}

\noindent \textbf{Different subject-aware T2I generation methods.}
We compare the image-driven editing results leveraging Custom Diffusion~\cite{CustomDiff} for reference subject learning with two other subject-aware T2I methods, \textit{i.e.}, Textual Inversion~\cite{TI}, and DreamBooth~\cite{dreambooth} and the visualization results are presented in Figure~\ref{fig:db}.
Given only one reference image, editing results generated with Custom Diffusion most closely resemble the reference image. 
Though the other two methods can generate similar categories and shapes, they do not match the reference image in texture. 
Therefore, in our paper, we ultimately select Custom Diffusion for reference subject learning.

\begin{figure}[!t]
    \centering
    \includegraphics[width=\linewidth]{sec/figure/cls.pdf}
    \caption{Visualization of different class words used in local editing prompt.}
    \label{fig:cls}
\end{figure}

\begin{figure}[!t]
    \centering
    \includegraphics[width=\linewidth]{sec/figure/db.pdf}
    \caption{Comparison between different subject-aware T2I generation methods for reference subject learning.}
    \label{fig:db}
\end{figure}

\begin{figure}[!t]
    \centering
    \includegraphics[width=\linewidth]{sec/figure/voxe.pdf}
    \caption{Qualitative comparison with Vox-E.}
    \label{fig:voxe}
\end{figure}

\begin{figure}[!t]
    \centering
    \includegraphics[width=\linewidth]{sec/figure/fail.pdf}
    \caption{Failure cases.}
    \label{fig:fail}
\end{figure}

\section{More Visualization Results}

\noindent \textbf{Comparison with Vox-E.}
We present qualitative comparison with Vox-E~\cite{voxe} in Figure~\ref{fig:voxe}.
Our method generates more realistic editing results than Vox-E. 
In the 1st row, the editing results by VoX-E maintain the shape of the pinecone and have an unnatural color. 
Besides, some odd color artifacts can be observed in both rows of Vox-E's edits, due to Vox-E's attention-based post-blending strategy, and our editing results strike a balance between text prompt alignment and background preservation.

\noindent \textbf{More qualitative results.}
We provide more image-driven and text-driven editing results in Figure~\ref{fig:m_img} and Figure~\ref{fig:m_text} respectively.
% We have also included video editing results in the [``video results'' folder], which provides dynamic visualization of editing results.
We have also included video editing results at \url{https://customnerf.github.io/}, which provides dynamic visualization of editing results.
% \textcolor[rgb]{0,0,1}{
% To highlight the advantages of our method, we evaluate it mostly on the challenging object replacement editing tasks. However, our method can perform far more editing tasks, such as texture editing, object insertion, style transfer, etc, which are presented in Fig. 1(e). For object replacement, the new object is not necessarily semantically related to the original one but should have a similar structure. Significant structural differences may lead to a blended structure in the edited object, as we have discussed in the failure cases (Figure 5 of Supp.). For structural differences within a certain range, our method significantly outperforms IN2N as shown in Fig. 1(f).
% }

\noindent \textbf{Failure cases.}
In addition to the experimental results above, we also present the failure cases of CustomNeRF in Figure~\ref{fig:fail}. 
For instance, in the first row, as the Custom Diffusion cannot always generate images with the subject identical to those in the reference image, the edited scene shows the dog's clothing different from that in the reference image.
In the second row, due to the considerable shape difference between a hat and a hamburger, the replaced hamburger takes on an inverted shape, larger at the bottom and smaller at the top, similar to the hat's structure.

\begin{figure*}[!htbp]
    \centering
    \includegraphics[width=.95\linewidth]{sec/figure/m_img.pdf}
    \caption{More visualization results of image-driven editing.}
    \label{fig:m_img}
\end{figure*}

\begin{figure*}[!htbp]
    \centering
    \includegraphics[width=.95\linewidth]{sec/figure/m_text.pdf}
    \caption{More visualization results of text-driven editing.}
    \label{fig:m_text}
\end{figure*}
