# Supplementary material for: Re-Align: Structured Reasoning-guided Alignment for In-Context Image Generation and Editing
Source: arXiv:2601.05124 source file (2026-01-08)
Supplement: Supplementary file 2 [file appendix.tex]

\clearpage
\begin{appendices}

\end{appendices}
